# Supplementary material for: Forecasting Interactive Dynamics of Pedestrians with Fictitious Play
Source: arXiv:1604.01431 source file (2017-03-28)
Supplement: Supplementary file 1 [file appendix1.tex]

\subsection{Forecasting Period and Forecasting Window Size}

We now take a deeper look at the parameters that define the recursive reasoning parameters of the fictitious play algorithm. How far into the future (forecasting window) should the model predict others' movements? How often (forecasting period) should each agent update predictions? In order to better understand how forecasting window size $W$ and forecasting period $\tau$ affect the performance of our approach, we perform grid search over the two parameters on the Town Centre dataset, with the estimated speed information included.

From Table \textcolor{red}{4}, we can see that given a fixed forecasting window size $W$, NLL and SCR always increase (gets worse) as the forecasting period $\tau$ becomes larger. This phenomenon implies that no matter how far one sees into the future, it is better to predict the actions of others as frequent as possible. This result is reasonable since a larger $\tau$ means we assume no changes in the dynamics of the scene over a longer period of time.
As for fixing $\tau$ and increasing $W$, SCR decreases initially and then increases with $W$ as expected. This is reasonable since at first the more future steps one forecasts, the more conservative one would be, and therefore less likely to collide with another person. However, as $W$ becomes very large, all agents become overly conservative and may result in collision. Note that NLL does not have a consistent relationship with $W$, and the breaking point (where scores change from decreasing to increasing) for NLL and SCR is different with various $\tau$. However, in most cases both metrics reach their minimum when $W = 3$. This result to some extent implies that pedestrian in our datasets tends to forecast three steps into the future of others. 

%\begin{comment}
\begin{table}[tb]
\label{tab:gridsearch}
\scriptsize
 \begin{center}
\centering
 \scalebox{1}{
 \begin{tabular}{|c|c|c|c|c|c|}
 \hline
\multicolumn{2}{|c|}{\multirow{2}{*}{NLL}} &\multicolumn{4}{c|}{Forecasting Period}\\\cline{3-6}
 \multicolumn{2}{|c|}{} & 1 & 3 & 5 & 7\\\hline
 \parbox[t]{2mm}{\multirow{4}{*}{\rotatebox[origin=c]{90}{\small W}}} 
 & 1 &14.6947    &14.7970	    &15.7602	&15.909\\
 & 3 &{\bf 10.892}	&15.5158	&15.7619    &15.7657\\
 & 5 &13.3353	&15.7070	    &15.5890  &16.1033\\
 & 7 &14.2277	&15.6970	    &15.7940	    &16.2070\\
 \hline
  %\end{tabular}
  %}
  %\scalebox{1}{
  %\begin{tabular}{|c|c|c|c|c|c|}
 \hline
\multicolumn{2}{|c|}{\multirow{2}{*}{SCR}} &\multicolumn{4}{c|}{Forecasting Period}\\\cline{3-6}
 \multicolumn{2}{|c|}{} & 1 & 3 & 5 & 7\\\hline
 \parbox[t]{2mm}{\multirow{4}{*}{\rotatebox[origin=c]{90}{\small W}}} 
 & 1 	&0.0735	&0.1187	&0.167	&0.1830\\
 & 3 &{\bf0.0493}	&0.1199	&0.1390  &0.1606\\
 & 5 &0.0934	&0.1200	&0.1287 &.1460\\
 & 7 &0.1052	&0.1221	&0.1320	&0.1427\\
 \hline
 \end{tabular}
 }
 \end{center}
 \caption{Performance of our model using various fictitious play parameters}
 \vspace{-3mm}
 \end{table}
 %\end{comment}

\subsection{Feature Analysis}
We further evaluate the effects of the features used in our proposed model. Results on the Zara dataset and the LIDAR Trajectory dataset using different features are respectively shown in Table \ref{tab:feature-analysis-zara} and Table \ref{tab:feature-analysis-lidar}. With the inclusion of the social compliance feature, our proposed model better explains the interactions between multiple pedestrians. We note that our approach is a generalization of \cite{kitani2012activity} to the multi-agent scenario. If there is only one agent, there will be no social compliant feature and our proposed model will reduce to nMDP where $n = 1$.

\begin{table}[t]
%\vspace{-0.5cm}
\centering
\scalebox{0.75}{
\begin{tabular}{|c|cccc||c|c|c|c|}
\hline
&$f_{occ}$ & $f_{dog}$ & $f_{bod}$ & $f_{soc}$ &nMDP\cite{kitani2012activity} &MDPCV	&mTA\cite{pellegrini2009you}&FP\\
\hline
\hline
\multirow{4}{*}{\rotatebox[origin=c]{90}{NLL}}
&\checkmark & \checkmark & & &48.23 &47.63 &48.23 &48.23\\
&\checkmark & \checkmark & \checkmark& &46.54 &46.95 &46.54 &46.54\\
&\checkmark & \checkmark & &\checkmark &48.23  &47.63 &43.82 &42.43 \\
&\checkmark & \checkmark & \checkmark& \checkmark&46.54 &46.95 &43.38 &42.14\\
\hline
\end{tabular}
}
\centering
\scalebox{0.75}{
\begin{tabular}{|c|cccc||c|c|c|c|}
\hline
&$f_{occ}$ & $f_{dog}$ & $f_{bod}$ & $f_{soc}$ &nMDP\cite{kitani2012activity} &MDPCV	&mTA\cite{pellegrini2009you}	&FP \\
\hline
\hline
\multirow{4}{*}{\rotatebox[origin=c]{90}{SCR}}
&\checkmark & \checkmark & & &0.150 &0.137 &0.150 &0.150\\
&\checkmark & \checkmark & \checkmark& &0.144 &0.114 &0.144 &0.144\\
&\checkmark & \checkmark & &\checkmark &0.150 &0.137  &0.086 &0.037\\
&\checkmark & \checkmark & \checkmark& \checkmark&0.144 &0.114 &0.065 &0.013\\
\hline
\end{tabular}
}
\caption{Contribution of each feature to our model on Zara.}
\label{tab:feature-analysis-zara}
%\vspace{-0.3cm}
\end{table}

\begin{table}[t]
%\vspace{-0.5cm}
\centering
\scalebox{0.75}{
\begin{tabular}{|c|cccc||c|c|c|c|}
\hline
&$f_{occ}$ & $f_{dog}$ & $f_{bod}$ & $f_{soc}$ &nMDP\cite{kitani2012activity} &MDPCV	&mTA\cite{pellegrini2009you}&FP\\
\hline
\hline
\multirow{4}{*}{\rotatebox[origin=c]{90}{NLL}}
&\checkmark & \checkmark & & &95.84 &95.66 &95.84 &95.84\\
&\checkmark & \checkmark & \checkmark& &92.56 &93.17 &92.56 &92.56\\
&\checkmark & \checkmark & &\checkmark &95.84 &95.66 &92.12 &88.72\\
&\checkmark & \checkmark & \checkmark& \checkmark&92.56 &93.17 &91.97 &87.47\\
\hline
\end{tabular}
}
\centering
\scalebox{0.75}{
\begin{tabular}{|c|cccc||c|c|c|c|}
\hline
&$f_{occ}$ & $f_{dog}$ & $f_{bod}$ & $f_{soc}$ &nMDP\cite{kitani2012activity} &MDPCV	&mTA\cite{pellegrini2009you}	&FP \\
\hline
\hline
\multirow{4}{*}{\rotatebox[origin=c]{90}{SCR}}
&\checkmark & \checkmark & & &0.224 &0.208 &0.224 &0.224\\
&\checkmark & \checkmark & \checkmark& &0.197 &0.173 &0.197 &0.197\\
&\checkmark & \checkmark & &\checkmark &0.224 &0.208 &0.113 &0.031 \\
&\checkmark & \checkmark & \checkmark& \checkmark&0.197 &0.173 &0.082 &0.022\\
\hline
\end{tabular}
}
\caption{Contribution of each feature to our model on LIDAR Trajectory dataset}
\label{tab:feature-analysis-lidar}
%\vspace{-0.3cm}
\end{table}

\begin{comment}
 \subsection{Destination Forecasting}

In previous sections, we have assumed that the destinations of each pedestrian is known to understand the role of social compliance features and to decouple the effect of uncertain about the goal. In many situations, the final destination of a pedestrian is not known and needs to be inferred. Following~\cite{kitani2012activity}, we densely generate potential goals on the map and perform the same forecasting experiment.

We evaluate the performance of the our destination forecasting model on the Town Centre dataset and the Zara dataset. The only information used is the start locations for each pedestrian. Results show that our FP based approach consistently outperforms others even without knowing the destinations ahead of time. The absolute performance of all models degrade due to uncertainty about the goal. From Table \textcolor{red}{5} we observe that mLTA still performs the second best, while nMDP still performs the worst. Together with Table \textcolor{red}{1}, experimental results show that our model which models the interplay and visual evidence outperforms the baseline models.

\end{comment}
